# Supplementary material for: StyleHEAT: One-Shot High-Resolution Editable Talking Face Generation via Pre-trained StyleGAN
Source: arXiv:2203.04036 source file (2022-03-17)
Supplement: Supplementary file 1 [file appendix.tex]

% \section{Network Architectures}
% \revised{Table ~\ref{tbl:net_sof} shows detailed specifications of each sub-module in the neural \textit{SOF} representation described in Sec.~\ref{SOF Network Approximate} of the main manuscript. Table ~\ref{tbl:net_siw} shows detailed network specifications for the texture modeling described in Sec.~\ref{sec:siw stylegan} of the main manuscript.}

% \definecolor{Blue}{rgb}{0.00,0.00,1.00}
% \begin{table}[ht]
% % \color{Blue}
% \begin{tabular}{cccc}
% \toprule\hline
% & \textbf{Layer}  & \textbf{Channels} & \textbf{Input} \\ \hline
% \multirow{3}{*}{\textbf{T}} 
%   & $fc_{0\_0}$   & 3/256  & point location $x$ \\
%   & $fc_{0\_1}$   & 256/256  & $fc_{0\_0}$ \\ 
%   $\Theta$ & $fc_{0\_2}$   & 256/256  & $fc_{0\_1}$ \\ \hline
% \multirow{5}{*}{\textbf{\textit{RayMarcher}}} 
%   & $fc_{1\_0\_l}$   & 256/256   & $fc_{0\_2}$ \\
%   & $fc_{1\_0\_b}$     & 3/256   & ray\_dir $\vec{d}$ \\
%   & $fc_{1\_i\_l}$   & 256/256   & $fc_{1\_{(i-1)}\_l}+fc_{1\_{(i-1)}\_b}$ \\
%   $i \in [1,5]$ & $fc_{1\_i\_b}$     & 3/256   & ray\_dir $\vec{d}$ \\
%   & $fc_{1\_6\_l}$   & 256/1     & $fc_{1\_5\_l}+fc_{1\_5\_b}$ \\
%   & $fc_{1\_6\_b}$     & 3/1     & ray\_dir $\vec{d}$ \\
%   &&& $fc_{1\_6\_l} + fc_{1\_6\_b}$\\\hline
% \multirow{3}{*}{\textbf{\textit{Classifier}}} 
%   & $fc_{2\_0}$    & 256/256    & $fc_{0\_2}$ \\
%   & $fc_{2\_1}$    & 256/256    & $fc_{2\_0}$ \\
%  $\Phi$  & $fc_{2\_2}$    & 256/256    & $fc_{2\_1}$ \\
%   & $fc_{2\_3}$   & 256/20     & $fc_{2\_2}$ \\
%   &&&$fc_{2\_3}$\\\hline
% % \multicolumn{5}{l}{} \\
% % \bottomrule

% \bottomrule
% \end{tabular}
% \caption{\revised{\textbf{Layer specifications for the neural \textit{SOF} representation.} \textit{fc} denotes a fully-connected layer with \textbf{\textit{Layer Normalization}} and \textbf{\textit{ReLU}} activation.}}
% \label{tbl:net_sof}
% \end{table}


% \begin{table}[ht]
% % \color{Blue}
% \begin{tabular}{ccccc}
% \toprule\hline

% & \textbf{Layer} & \textbf{Channels}& \textbf{s} & \textbf{Input} \\ \hline
% \multirow{15}{*}{\textbf{\textit{SIW-StyleGAN}}} 
%   & $Conv_{0\_0}$ &  16 & 2 & $\mathcal{M}$\\
%   & $Conv_{0\_1}$ &   16 &  1  & $Conv_{0\_0}$\\
% $i \in [1,3]$ & $Conv_{i\_0}$ &  $16\times2^i$ & 2 & $Conv_{(i-1)\_0}$\\
%   & $Conv_{i\_1}$ &   $16\times2^i$ &  1  & $Conv_{i\_0}$\\
  
%     & $\Psi_0$ &  512 &  $1/2$ & $z^t, Conv_{3\_1}$\\
% $j \in [1,3]$    & $\Psi_j$ &  512 &  $1/2$ & $z^t, \Psi_{j-1}$\\
% & $\Psi_4, \mathcal{N}$ &  512 &  $1/2$ & $z^t, \Psi_3, \mathcal{M}, \mathcal{P}$\\
% & $\Psi_5, \mathcal{N}$ &  256 &  $1/2$ & $z^t, \Psi_4, \mathcal{M}, \mathcal{P}$\\
% & $\Psi_6, \mathcal{N}$ &  128 &  $1/2$ & $z^t, \Psi_5, \mathcal{M}, \mathcal{P}$\\
% & $\Psi_7$ &  64 &  $1/2$ & $z^t, \Psi_6, \mathcal{P}$\\
% & $\Psi_8$ &  32 &  $1/2$ & $z^t, \Psi_7, \mathcal{P}$\\
% & $\Psi_9$ &  3 &  $1/2$ & $z^t, \Psi_8, \mathcal{P}$\\
% \hline
% \bottomrule
% \end{tabular}

% \caption{\revised{\textbf{Network architecture for texture modeling (SIW-StyleGAN).} \textbf{s} denotes stride size and $\mathcal{M}$ denotes the semantic segmentation map. $z^t \in \mathcal{R}^{2\times512}$ and $\Psi$ is the texture style modulation function as mentioned in Sec.~\ref{sec:siw stylegan}. $\mathcal{N}$ is the spatially adaptive normalization layer while $\mathcal{P}$ is the style distance map for the mixed style training.}}
% \label{tbl:net_siw}
% \end{table}
